# Supplementary material for: Gaussian3Diff: 3D Gaussian Diffusion for 3D Full Head Synthesis and Editing
Source: arXiv:2312.03763 source file (2023-12-19)
Supplement: Supplementary file 1 [file X_suppl.tex]

\clearpage
\setcounter{page}{1}
\maketitlesupplementary

In this supplementary material, we provide additional details regarding the implementations and additional results. We also discuss the limitations of our model, and provide a supplementary HTML page showing animated results.

\section{Implementation Details}

\subsection{Auto-decoder Loss Functions}
\heading{Reconstruction Loss}
We first briefly introduce the supervision we adopt in image reconstructions in both training stages~\ref{sec:training_decoder}.
Note that all those supervisions are imposed on both the raw-3D low-res predictions and super-resolution module high-res outputs.
First, we utilize the pixel-wise $\loss_1$ loss,
% \vspace{-1.15mm}
\begin{equation}
    \loss_{\text{1}}\left ( \image \right ) = || \image - \imagePredicted ||_1 \enspace .
\end{equation}

% \vspace{-1.15mm}
In addition, to learn perceptual similarities, we use the LPIPS~\cite{zhang2018perceptual} 
loss, which has been shown to better preserve image quality compared to the more standard perceptual loss:
% ~\cite{johnson2016perceptual}:
\begin{equation}
    \loss_{\text{LPIPS}}\left ( \image \right ) = || F(\image) - F(\imagePredicted)||_2 \enspace,
\end{equation}
where $F(\cdot)$ denotes the perceptual feature extractor.

Moreover, we render the multi-view depths from Panohead~\cite{An_2023_CVPR} samples for supervision, as in DepthNeRF~\cite{kangle2021dsnerf}:

\begin{equation}
    \loss_{\text{depth}}\left ( \image \right ) = || D(\image) - D(\imagePredicted)||_2\enspace,
\end{equation}
where $D(\cdot)$ denotes the depth corresponding to the input image, which are computed in volumetric rendering.

Finally, a common challenge when handling the specific task of encoding facial images is the preservation of the input identity. To tackle this, we incorporate a dedicated recognition loss measuring the cosine similarity between the output image and its source, 
% \vspace{-1.25mm}
\begin{equation}
    \loss_{\text{Id}}\left (\image \right ) = 1-\left \langle R(\image),R(\imagePredicted)) \right \rangle \enspace,
\end{equation}
where $R$ is the pretrained ArcFace~\cite{deng2019arcface} network.

In summary, the overall reconstruction loss is the weighted summation of the loss functions described above:
\begin{equation}
    \loss_{\text{rgb}} = 
    \loss_{\text{1}} + \loss_{\text{LPIPS}} +  \lambda_{\text{depth}}\loss_{\text{depth}} +\lambda_{\text{Id}} \loss_{\text{Id}}
    \enspace.
\end{equation}
where we set $\lambda_{\text{depth}}=0.1$ and $\lambda_{\text{Id}}=0.1$. In the first training stage, the auto-decoder is optimized without the SR module, we set $\lambda_{\text{Id}}=0$.

\heading{Gaussian Regularization Loss}
Inspired by existing studies on 3D local representations~\cite{zhang2023nerflets,genova2019deep,Lombardi21MVP}, we impose the following regularization terms to stabilize the Gaussian training and better mirror the structure of the scene.
We first impose $\calL_{\text{cov}}$, the coverage loss which penalizes the $L_1$ norm of the Gaussian influence values (RBF) at the sample locations and encourages sparsity where possible:
\begin{equation}
\calL_\text{cov}(\gaussian, \point)=
\lambda_{\text{cov}}
\frac{1}{K}
\sum_{k}^{K} g_i(\bfx)
\enspace ,
\end{equation}

where $g$ is the RBF value at query point $\bfx$ influenced by Gaussian $\gaussian$ and $K=3$ specifies the number of nearest Gaussians that contribute to $\bfx$.

To prevent the optimized ellipsoid from growing too large, we penalize the ellipsoid volume size by:
\begin{equation}
\calL_\text{vol}(\gaussian)=
% \frac{4\pi}{3N}
% \sum_{i=1}^{N}
\lambda_{\text{vol}}
% \lambda_{\text{coverage}}
\frac{4\pi}{3}
% \sum_{i=1}^{N}
{\prod_j^3(\Sigma^{-1})_{j,j}} \enspace ,
\end{equation}
where $(\Sigma^{-1})_{j,j}$ parameterizes the 3 axis-aligned radiis, which are the reciprocal of the variance along each principal axis.

Besides, we calculate the silhouette of a given image to encourage a cleaner background:
\begin{equation}
    \loss_{\text{silhouette}}\left ( \image \right ) = \lambda_{\text{silhouette}}|| M(\image) - M(\imagePredicted)||_2\enspace,
\end{equation}
where $M(\cdot)$ denotes the silhouette mask of the given image.

We also impose a Total-Variance smoothness term over the Gaussians to encourage nearby Gaussians on the UV should change smoothly:
\begin{equation}
\calL_\text{TV}(\gaussian)=
\lambda_{\text{TV}}
\frac{1}{N}
\sum_{h,w}^{N}
{\abs{\gaussian_{h+1,w}-\gaussian_{h,w}} +\abs{\gaussian_{h,w+1}-\gaussian_{h,w}}} \enspace ,
\end{equation}
where $N$ is the UV map size and $h,w$ is the spatial UV map index.

Furthermore, we ensure that the optimized Gaussian centers remain aligned with the initial 3DMM registration by employing a regularization term that penalizes deviations from the initialized 3DMM mesh vertices $\mathbf{v}$, as expressed in the following loss function:
$$
\mathcal{L}_{\text{mesh}}(\gaussian) =
\lambda_{\text{mesh}}
\frac{1}{N}
\sum_{h,w}^{N}
{\big|\big| \mathbf{v}_{h,w} -  \bfmu_{h,w} \big|\big|_2^2} \enspace,
$$
as in the approach of \cite{lombardi2018DAM}.

The final Gaussian regularization loss reads as the weighted summation of all the terms listed above:
\begin{align}
    \label{eq:losses_reg}
    \calL_\text{reg} = \calL_{\text{cov}}  + \calL_\text{vol} + \loss_{\text{silhouette}} + \calL_\text{TV} + \calL_\text{mesh} \enspace, 
\end{align}
where we set 
$\lambda_{\text{cov}}=0.001$,
$\lambda_{\text{tanh}}=0.1$,
$\lambda_{\text{silhouette}}=1$,
$\lambda_{\text{vol}}=1$,
$\lambda_{\text{TV}}=0.1$,
and $\lambda_{\text{mesh}}=0.01$ as the defined loss weights.

\heading{Code Prior Loss}
For optimizing auto-decoder $\decoder$, following DeepSDF~\cite{park2019deepsdf} we have
\begin{equation}
\mathcal{L}_{\text{code}} =  
\lambda_{\text{code}}
\frac{1}{\sigma^2} \lVert \zz \rVert_2^2 \enspace ,
\end{equation}
where in the latent shape-code space, we assume the prior over codes $p(\zz_i)$ to be a zero-mean multivariate-Gaussian with a spherical covariance $\sigma^2 I$. We initialize $\zz$ from $\mathcal{N}(0,0.01^2)$ and set $\lambda_{\text{code}}=1e-4$ following DeepSDF.

\subsection{Data Preparation}
\heading{Panohead Data Generation}
\begin{figure}[t]
  \includegraphics[width=0.5\textwidth]{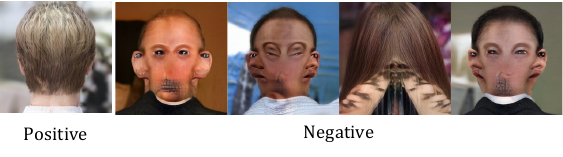} 
  \vspace{-4mm}
  \caption{\textbf{Visualization of positive and negative samples from Panohead.} The display includes one positive sample and four negative samples here. The positive sample process a ``human front face'' score of $2.16e-04$, while all the negative samples process scores $\ge 0.5$.}
\label{fig:clip-filter}
\end{figure}
Due to its ability to generate high-quality full-head 3D portraits, we adopt Panohead~\cite{An_2023_CVPR} as our 3D data source~\cite{zhang21datasetgan}.
Though the tri-grid design greatly alleviates the Jenus problem~\cite{poole2022dreamfusion} compared with tri-plane~\cite{Chan2021EG3D}, in practice we still find around $30\%$ among Panohead synthesized samples are likely to fail, as shown in Fig.~\ref{fig:clip-filter}.
We observed that these samples even cannot be reconstructed well and greatly poison the auto-decoder's performance.
Therefore, we filter those samples with CLIP~\cite{Radford2021CLIP}, where we calculate the CLIP score of the input back head image with two text prompts ``human front face" and ``back of human head" and calculate the normalized softmax probability.
We leave all samples with the ``human front face" score $<0.007$ for training.

\heading{Registration}
\label{sec:registration} 
Due to the scale differences between 3D Morphable Models (3DMMs) and 3D human heads synthesized from Panohead~\cite{An_2023_CVPR}, direct fitting of a 3DMM to multi-view images with pre-defined camera poses used in data generation is not feasible~\cite{li2017learning}. To overcome this challenge, we employed a 3DMM fitting algorithm to simultaneously estimate 3DMM parameters and camera poses from multi-view images. Subsequently, a homogeneous transformation with scaling is computed to align the estimated camera poses with the pre-defined camera poses. This transformation is then applied to the fitted 3DMM mesh to transform it into the Panohead coordinates.

\subsection{Training Details}
\heading{Auto Decoder}
\label{sec:training_decoder} 
We adopted AdamW optimizer with no weight decay for all the experiments,
and set $lr=0.05$ for optimizing $\zz$, $lr=0.0025$ for optimizing autodecoder $\decoder$ and $lr=1e-5$ for optimizing Gaussians and $lr=5e-2$ for optimizing a tiny $2$-layer rendering MLP with $8\times32\times4$ shape. 
We decay all the learning rates at 100k steps by a factor of $0.5$.

We first train the autodecoder using $64\times64$ raw renderings from Panohead with batch size $30$ for 250K iterations and achieve PSNR around $28$db. For scalability, for each data point, we randomly crop a $36\times36$ patch for supervision. 
We augment the background color to white to encourage better foreground-background disentanglement.
In the next stage, we cascade a pre-trained ESRNet~\cite{wang2018esrgan} after the autodecoder to upsample the $64\times64$ renderings, resulting in high-resolution synthesis at $256\times256$. 
$\mathcal{L}_\text{Id}$ is only imposed during the second stage.
We set the learning rate for ESRNet with $1e-4$ and jointly train both models with batch size $4$ for another 250k iterations. The overall training takes around $6$ days on two RTX A6000 GPUs.
The stored autodecoder checkpoint occupies a space of $66.96$ MiB, while the ESRNet consumes $63.94$ MiB.

\heading{Diffusion Models}
% We follow the diffusion model implementation of Imagen~\cite{saharia2022photorealistic} and list the details in Tab.~\ref{tab:diffusion-params}.
% % 
% Before training, we set the expression of the reconstructed 3D Gaussians to neutral, so that the generated results can be directly driven by adding the expression offsets~\cite{FLAME:SiggraphAsia2017}.
% % 
% We train the diffusion model using Jax on $16$ A100 GPUs for $500K$ iterations, which takes around $5$ days.
We adhere to the diffusion model implementation as outlined in Imagen~\cite{saharia2022photorealistic}, and the specific details are enumerated in Tab.~\ref{tab:diffusion-params}.
Note that we normalize the Gaussians and payload features to $[-1,1]$ for better diffusion learning.
Besides, we set the expression of the reconstructed 3D Gaussians to the neutral state. 
This ensures that the generated outcomes can be directly animated by adding expression offsets, as per the methodology proposed in FLAME~\cite{FLAME:SiggraphAsia2017}.
We train the diffusion model using Jax on $16$ A100 GPUs for $500K$ iterations, which takes around $5$ days.

\begin{table}[h]
\begin{center}
\scalebox{0.85}{%
\setlength{\tabcolsep}{0.19em}
\begin{tabular}{lcccccc}
\toprule
Diffusion Model Details \\
% & \multicolumn{3}{c}{Unconditional} & \multicolumn{3}{c}{Reconstruction} \\
% \cmidrule(lr){2-4} \cmidrule(lr){5-7}
% & Cars (full) & Cars (3-view) & Tables (full) & Cars (full) & Cars (3-view) & Chairs (full) \\
\midrule
Learning Rate &  $2e-5$ \\
Batch Size &  $96$ \\
Optimizer &  ADAM \\
$\gaussian_0$ shape &  (9+3$\times$8)$\times$256$\times$256 \\
U-Net base channels &  256 \\
U-Net channel multiplier &  1, 1, 2, 2, 4, 4 \\
U-Net res block &  2 \\
U-Net attention resolutions &  32, 16, 8 \\
U-Net attention head &  4 \\
U-Net attention head channels &  64 \\
U-Net norm layer type &  GroupNorm \\
% U-Net dropout & 0.0 & 0.0 & 0.0 & 0.1 & 0.1 & 0.1 \\ 
Diffusion steps &  1000 \\
Noise schedule &  Cosine \\
Clip Input $[-1,1]$ & True \\
\midrule
normalizing Gaussian centers  & \lstinline{(x + 0.12) * 2} \\
normalizing Gaussian rotations  & \lstinline{x / math.pi} \\
normalizing Gaussian radii  & \lstinline{(x.abs().clip(0, 0.15) - 0.06) * 10}\\
normalizing Gaussian payload  &  \lstinline{tanh(x)} \\
\bottomrule
\end{tabular}}
\end{center}
\caption{Hyperparameters and architecture of diffusion model $f_\theta$. Additionally, it is worth noting that we also normalize $\gaussian_0$ to range $[-1,1]$ to enhance diffusion training, employing the normalization function detailed above.}
\label{tab:diffusion-params}
\end{table}

% \subsection{Profiling}
% \heading{Model Size}
% \yslan{later.}
% \heading{Model Latency}

\section{More Analysis}
\subsection{More Ablation Studies}
\heading{Selection of $K$ Nearby Gaussians for Blending}
\begin{table}[tp]
\centering
\small
{
% \caption{\textbf{Quantitative ablation of $K$ in Gaussian Blending.} Larger $K$ yields better reconstruction at an extra computational cost. BS denotes batch size.} 
\caption{\textbf{Quantitative Ablation of $K$ in Gaussian Blending.} 
We evaluate the reconstruction results at $20K$ iterations.
Increasing the value of $K$ improves the quality of reconstruction, albeit with an associated increase in computational resources. 
Nevertheless, beyond $K$=3, a decline in performance is observed, indicative of potential undertraining of the model.
BS denotes batch size.}
\vspace{-2mm}
\label{tab:abla:k}
\resizebox{\linewidth}{!}{
\begin{tabular}{l@{\hspace{3mm}}ccccc}
\toprule
$K$ value & PSNR  $\uparrow$ &  MAE $\downarrow$ &   VRAM(MiB)@BS=4 $\downarrow$  & Latency(s)/step $\downarrow$  \\
\midrule
$1$ & 27.72 $\pm$ 2.53 & 0.0421 $\pm$ 0.013 & 6886 & 0.4 & \\
$2$ & 27.92 $\pm$ 2.40 & 0.0412 $\pm$ 0.012 & 11508 & 0.53 & \\
$3$ & \textbf{28.39} $\pm$ 2.55 & \textbf{0.0392} $\pm$ 0.012 & 16124 & 0.67 & \\
$4$ & 28.28 $\pm$ 2.37 & 0.0400 $\pm$ 0.012 & 20774 & 0.8 & \\
$5$ &  28.25 $\pm$ 2.33 & 0.0395 $\pm$ 0.011 & 25402 & 0.87 & \\
\bottomrule
\end{tabular}}}
\vspace{0mm}
\end{table}
\begin{figure}[h!]
  \includegraphics[width=0.5\textwidth]{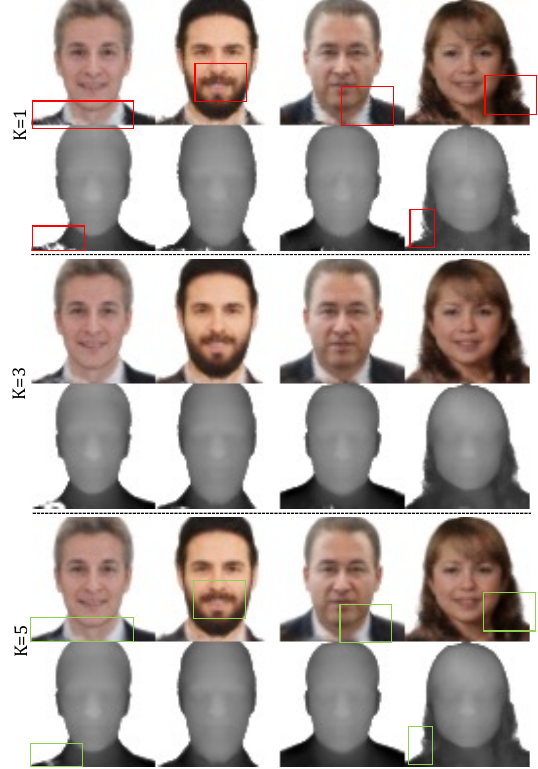}
%   \caption{\textbf{Qualitative Ablation of $K$ in gaussian Blending.} 
%   Though achieving comparative quantitative performance, smaller $K$ yields visually more noisy reconstruction, as we highlight in the \textcolor{red}{red box}. Setting $K=5$ improves smoothness, as shown in 
%   the \textcolor{green}{green box}. We adopt $K=3$ to balance the overall performance.
%   All results are obtained from auto-decoder $\decoder$ directly without super resolution.
%   }
\caption{\textbf{Qualitative Ablation of $K$ in Gaussian Blending.} Despite achieving comparable quantitative performance, a smaller $K$ results in visually noisier reconstruction, as shown in the \textcolor{red}{red box}. Setting $K=5$ enhances smoothness, as illustrated in the \textcolor{green}{green box}. We opt for $K=3$ to strike a balance in overall performance. All results are obtained directly from the auto-decoder $\decoder$, without employing super resolution.}
\label{fig:abla:knn}
\end{figure}
We investigate the choice of $K$ value in Gaussian blending and include the quantitative results in Tab.~\ref{tab:abla:k}. 
Specifically, we reconstruct $24$ instances using our method for $20k$ iterations using identical hyper-parameters except the $K$ and employing $\loss_\text{L1}$ loss. Note that we only compare the 64x64 outputs from the autodecoder, as the number of $K$ only affects the volumetric rendering.
As it can be observed, the reconstruction performance initially improves steadily with increasing $K$, as does the computational cost. This is because evaluating the RBF value of more Gaussians requires storing extra gradients and more computation.
Surprisingly, we did not observe quantitative performance gain after $K=3$. 
We further qualitatively compare the reconstruction differences in Fig.~\ref{fig:abla:knn}. Upon visual inspection, it is evident that smaller $K$ values produce noisier reconstructions in both color and depth, while increasing $K$ values gradually produce smoother and more complete results.
To trade off the overall performance, we adopt $K=3$ in our experiments. 
However, efficient training with larger $K$ is still worth exploring in future work.

\heading{Auto-Decoder Design}
Though existing 3D diffusion methods like Rodin~\cite{wang2023rodin} also adopt an auto-decoding design, it is noteworthy that only a shallow rendering MLP is reused across instances.
This design requires the learning of a shared decoder across hundreds of instances, followed by fitting each 3D object with the shared frozen decoder.
In our ablation study, we specifically investigate the use of a shared convolutional decoder $\decoder$ in Fig.~\ref{fig:abla:autodecoder}.
Specifically, we conduct texture transfer and expression editing experiments on overfitted samples where no shared auto-decoder is used.
As illustrated, the interpolation and expression editing yield semantically inconsistent results when compared with Fig.~\ref{fig:tex-transfer}, such as the absence of teeth.
Moreover, adopting a convolutional decoder for fitting enhances scalability, allowing for optimizing $10,000$ instances using $2$ GPUs.
% 
% Please check the supplementary for the qualitative comparisons.

\begin{figure}[ht]
  \includegraphics[width=0.5\textwidth]{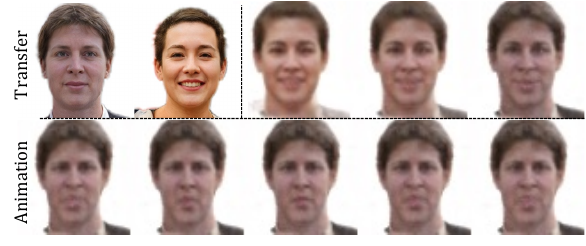} 
  \caption{\textbf{Ablation Study on autodecoder.} We first reconstruct two instances individually without a shared convolutional decoder and show the texture transfer in row$-1$, and animation results in row$-2$. Visually inspected, the baseline design lacks the ability to learn unseen missing features from other instances, \eg, teeth and diverse expression. Our design shows better generality and scalability.}
\label{fig:abla:autodecoder}
\end{figure}

\subsection{Limitations and Failure Cases}

\heading{Single-image Inversion}
\begin{figure}[t]
  \includegraphics[width=0.5\textwidth,]{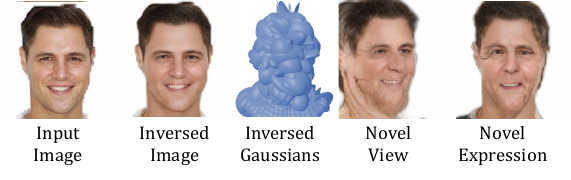} 
  \vspace{-6mm}
  \caption{\textbf{Single-view inversion on the pre-trained auto-decoder $\decoder$}
  We randomly sample one image from CelebA-HQ~\cite{CelebAMask-HQ} and conduct test-time optimization to find the corresponding Gaussians. while the input view can be plausibly reconstructed, 
%   the novel view and novel expression results have noticeable artifacts.
the results for novel views and expressions exhibit noticeable artifacts.
  }
\label{fig:inversion}
  \vspace{-2mm}
\end{figure}
% \begin{figure}[h!]
\begin{figure*}[ht]
  \includegraphics[width=1\textwidth]{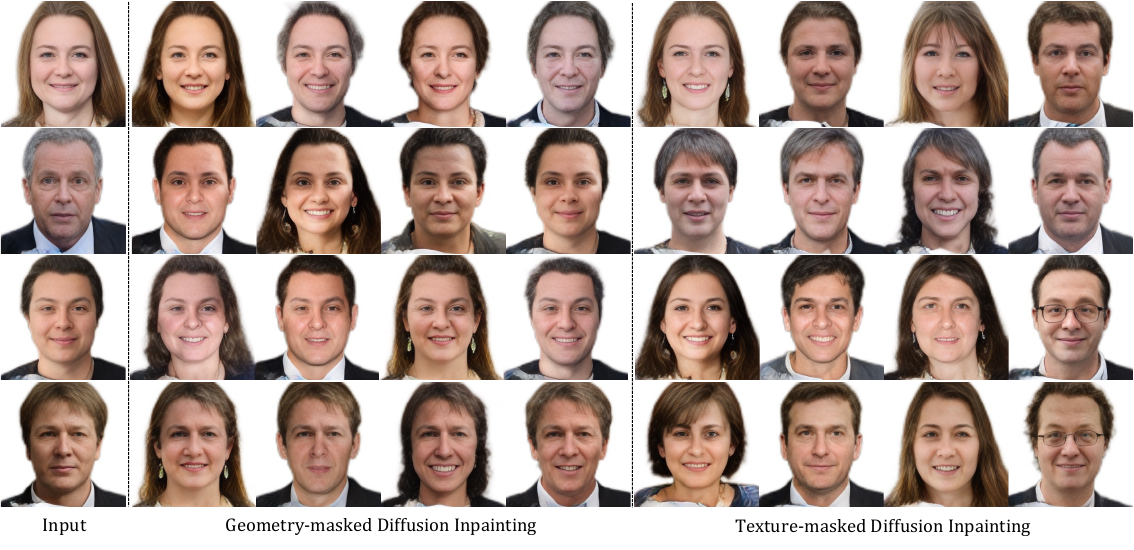}
  \caption{\textbf{Diffusion-based Inpainting given Geometry or Texture Mask.} 
%   We provide with the geometry-part (first $9$ channels of the $256\times256\times33$ of $\gaussian_0$) 
%   or the texture-part (last $24$ channels of the $256\times256\times33$ of $\gaussian_0$) of the upper face as the hints, and let the diffusion model $f_\theta$ in-paints the remaining. As shown in column $2-5$, all the generated results have identical upper-face shape, \eg, eyes and forehead layout, but with different textures; 
%   while all the texture-masked diffusion in-painted results (column $6-10$) have identical upper-face texture, \eg, hair and forehead color, but with different shape.
We provide either the geometry part (first $9$ channels of the $256\times256\times33$ tensor $\gaussian_0$) or the texture part (last $24$ channels of the $256\times256\times33$ tensor $\gaussian_0$) of the \emph{upper face} as hints, and take the diffusion model $f_\theta$ in-paints the remaining details. 
As illustrated in columns $2-5$, all the generated results exhibit an identical upper-face shape, including the layout of the eyes and forehead, but with different textures. Conversely, the diffusion-inpainted results with texture masks (columns $6-10$) showcase an identical upper-face texture, encompassing features such as hair and forehead color, while varying in shape.
  }
  \vspace{-2mm}
\label{fig:application:diffusion:geo-tex-inpaint}
\end{figure*}
% \end{figure}
Though we use multi-view images for reconstruction, here we include single-view inversion results in Fig.~\ref{fig:inversion}.
Specifically, we first register the 3DMM parameters following the procedures introduced in Sec.~\ref{sec:registration}.
Next, we adopt the SG2~\cite{abdal2019image2stylegan} inversion paradigm, which optimizes the latent code $\zz$ and Gaussians $\gaussian$ via the reconstruction loss.
As can be seen, though the input reconstruction is reasonable, the optimized Gaussians are noisy and the novel view synthesis and novel expressions are unsatisfactory.  
Therefore, how to conduct 3D Gaussian reconstruction from few-shot images is still open for future research.
Existing efforts in 3D-GAN inversion may also provide possible solutions, \eg, training a 3D-aware encoder~\cite{lan2022e3dge} or introducing pseudo depth loss~\cite{xie2022high}.

\heading{Dataset Bias}
A well-recognized challenge in deep generative models is the presence of bias, whereby the model exhibits a propensity to generate one gender more frequently than the other, or certain attributes become closely intertwined.
Given that our training data originates from Panohead, our model inherently inherits the bias issue present in the data. Specifically, we have observed a tendency for the generated females to exhibit a "smile" more frequently when compared to the generated male instances.
% A well-known problem in deep generative models is the bias issue, where the model tends to generate more gender than the other, or some attributes are closely entangled with each other.
% 
% Since our training data are from Panohead, the model we trained intrinsically inherits the data bias problem. Specifically, we observe that the generated females are more likely to be "smile" compared with the generated male instances.
% This can be intuitively seen in Fig.~\ref{fig:applicatin:id-transfer} column $4,6$ and $7$, where the expressions of the source identities are almost neutral, but the female reenactment results are still slightly smiling with their teeth visible.
This bias becomes apparent when examining Fig.~\ref{fig:applicatin:id-transfer} columns $4, 6$, and $7$, where the facial expressions of the source identities are predominantly neutral. Nevertheless, the female reenactment results still depict a subtle smiling expression, with visible teeth.

\heading{Jointly Training on Synthetic and  Real-world Dataset}
Real-world high-quality avatar dataset~\cite{wuu2022multiface} suffers from quantity and diversity, while the synthetic 3D-GAN synthetic samples suffer from resolution and expressions, where the raw 3D-renderings are usually limited to $64\times64$ with one expression available.
An open direction is to study how to marry the best of both data sources to establish a high-fidelity and diverse avatar system. 

\heading{Avatar-specific Design}
% \yslan{TODO: mouth, GAN loss etc. like in next3d,gfpgan.}
Presently, our training framework does not incorporate avatar-specific design elements, such as a mouth in-inpainting module in Next-3D~\cite{sun2023next3d}, landmarks supervision and face region-specific GAN loss as utilized GFPGAN~\cite{wang2021gfpgan}. 
Moreover, each training instance is constrained to a single expression.
Expanding our method to datasets and training designs tailored for
avatar-specific characteristics hold the potential for further performance improvement.

\begin{figure*}[ht]
  \includegraphics[width=1.0\textwidth]{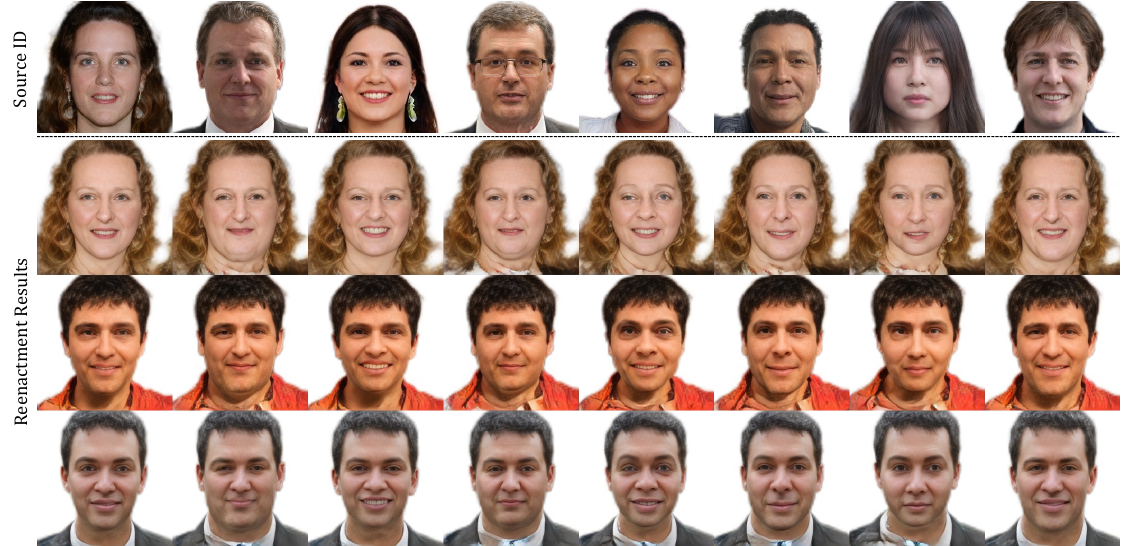} 
  \caption{\textbf{3DMM-based Editing}. We reenact $8$ random sampled source inputs (row-$1$) onto the targets (row-$2,3,4$) by driving the target Gaussians through the adjustment of the inner 3DMM mesh using the shape and expression codes from the source.
  The reenactment results preserve their original texture while adapting to the shape and expression of the source inputs.
  }
  \label{fig:applicatin:id-transfer}
\end{figure*}
\heading{Application on the General Scenes}
Currently, we only showcase the 3D Gaussians-based generation ability within the realm of 3D portraits. 
However, given the widespread use of UV map in the industry, expanding \nickname{} as a general 3D generative model is worth future investigation.

\section{More Application Results}
\heading{Shape-Texture Transfer}
\begin{figure*}[ht]
  \includegraphics[width=1.0\textwidth]{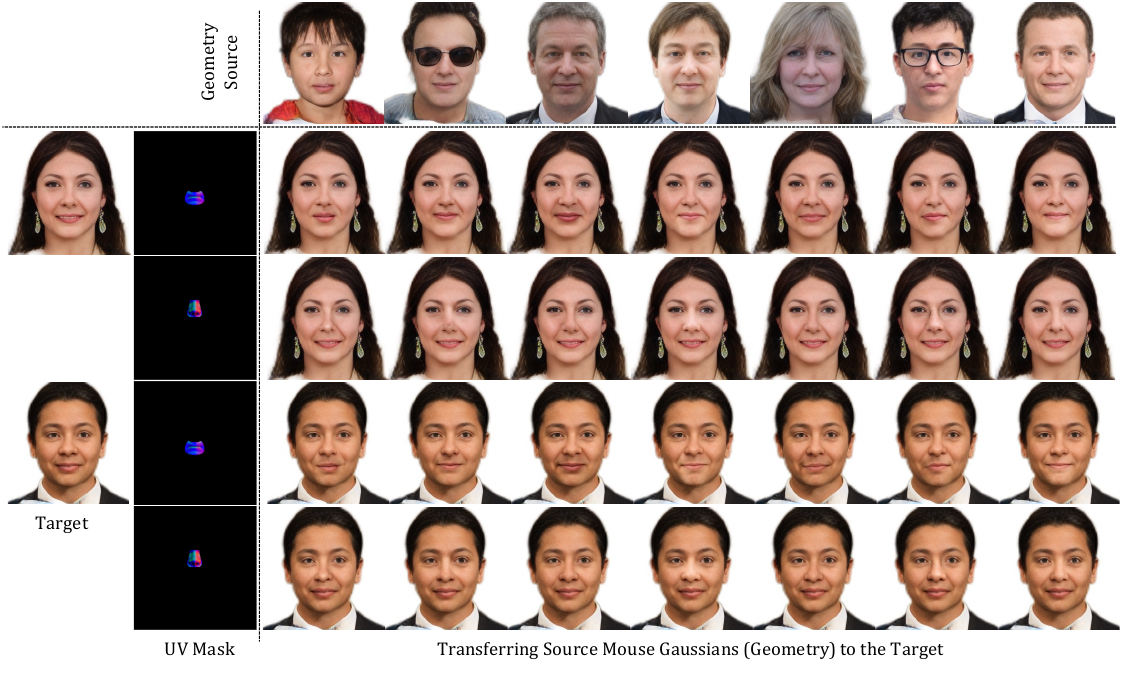} 
%   \includegraphics[]{example-image} 
%   \caption{\textbf{Regional Editing given UV Mask}. Thanks to the UV-space design, \nickname{} supports editing a specific semantics region defined on the UV map.
% %   
%  Here, we transfer the "nose" and "mouse" geometry shape from the source identities to the target and leaving the remaining areas unchanged.
% %   
%   Note that all the source and target identities here are diffusion-sampled.
%   }
\caption{\textbf{Regional Editing with UV Mask}. The UV-space design in \nickname{} enables the editing of specific semantic regions defined on the UV map.
  In this example, we transfer the geometry shapes of the "nose" and "mouth" from the source identities to the target while leaving the remaining areas unchanged.
  It is important to note that all the source and target identities presented here are diffusion-sampled.
  }

  \label{fig:applicatin:region-editing}
\end{figure*}
\begin{figure}[h]
  \includegraphics[width=0.5\textwidth]{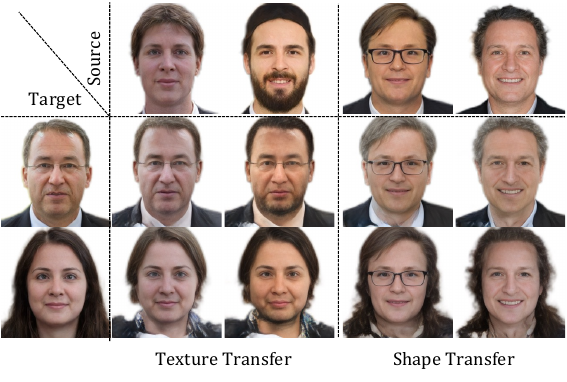} 
  \vspace{-6mm}
  \caption{\textbf{Shape Texture Transfer.} 
  Given two randomly sampled source identities, each serving as the source of texture (columns $1-2$) and shape (columns $3-4$), we transfer their corresponding information defined in the UV space to four targets.
Importantly, the transferred textures semantically adhere to the target shape; for instance, the beard in column $2$ varies according to the size of the Gaussians in that region.
Additionally, the texture source identity of column $1$ does not display teeth, while the transferred results do, illustrating that the autodecoder $\decoder$ learns a shared meaningful latent space.
These results, as evidenced in Fig.~\ref{fig:abla:autodecoder}, cannot be achieved via per-instance fitting.
}
\label{fig:tex-transfer}
\vspace{-4mm}
\end{figure}
\nickname{} naturally supports geometry-texture disentanglement, where Gaussians managing the geometry and attached local tri-planes determining the texture within a local region defined on the UV map. 
As illustrated in Fig.~\ref{fig:tex-transfer}, we conduct both shape and texture transfer by swapping the corresponding areas on the UV map from the source identity to the target.
Visually inspected, the texture-transferred identity inherits the texture characteristics from the source while maintaining the shape layout of the target, and the shape-transferred results maintain the layout of the source without affecting their textures.

\heading{3D Inpainting using Diffusion Model}
Our trained diffusion model supports 3D in-painting given geometry and texture mask individually.
We show both the geometry- and texture-based inpainting in Fig.~\ref{fig:application:diffusion:geo-tex-inpaint}. Both yield holistically reasonable results while keeping the corresponding inputs within the mask unchanged.
Note that there are still noticeable color changes between the inpainting boundaries, which could be addressed by introducing inpainting-specific training design~\cite{rombach2021highresolution}.

\heading{3DMM-based Editing}
\begin{figure}[h!]
  \includegraphics[width=0.5\textwidth]{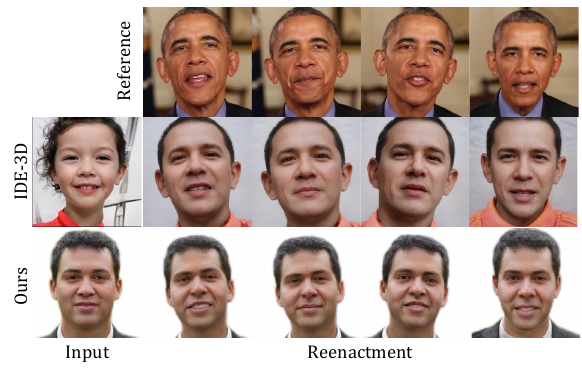} 
  \vspace{-6mm}
  \caption{\textbf{Comparison with IDE-3D on Reenactment.} Employing four reference images (row-$1$), we animate the identities synthesized by IDE-3D and our method to the target expression.
  Given IDE-3D's segmentation-based nature, utilizing a reference identity with a different shape inevitably alters the facial layout.
  Nevertheless, \nickname{} is build on a identity-and-expression disentangled modeling, facilitated by the underlying 3DMM, ensuring the preservation of the input identity through the reenactment process.
  }
\label{fig:baseline:ide3d}
\end{figure}
Thanks to the delicate design, \nickname{} marries the best of both the model-based 3DMM and neural representations through the rasterized UV space, and naturally supports 3DMM-based editing, \eg, avatar modeling by changing the shape and expression codes.
We show this ability by reenacting the shape and expression codes of given source identities onto the target reconstructed instances.
Specifically, we drive the learned Gaussians by adding the offsets between the positions of source identity vertices and initialized target identity vertices.
We reuse the identities included in Fig.4 in the main paper for simplicity.
As shown in Fig.~\ref{fig:applicatin:id-transfer}, the reenactment results maintain their original texture details but accurately follow the shape and expression of the given source input.
This application has the potential to facilitate avatar editing in game engines and media creation. 

\heading{Regional-based Editing}
In addition to global interpolation and transfer capabilities, \nickname{} provides support for region-based editing, allowing modification exclusively within the semantic region defined by the UV mask.
This functionality is illustrated in Fig.~\ref{fig:applicatin:region-editing}, where we showcase the transfer of corresponding source Gaussians (geometry) to the target, guided by the provided mask.
The transferred results exhibit the same shape as the source within the defined semantic region, while the remaining areas remain unchanged.
Benefiting from the thoughtful design of the UV space, regional editing consistently produces semantically consistent results when transferring between mouth/nose regions of varying sizes across different identities.
Furthermore, this demonstration underscores that \nickname{} can surpass 3DMM constraints, enhancing controllability and exhibiting significant potential for avatar personalization within game engines~\cite{metahuman}.

\section{More comparisons with Baselines}
% \heading{Next-3D}
% Animation.

% \heading{IDE-3D}
We include the qualitative reenactment comparison of IDE-3D~\cite{sun2022ide} to our method in Fig.~\ref{fig:baseline:ide3d}.
Both methods can accurately reflect the input expression in their reeactment results, although IDE-3D exhibits a deficiency to preserve the input identity, attributed to its segmentation-based animation paradigm.
This difference accounts for their inferior PCK performance compared to ours in the main paper.

Moreover, IDE-3D and FE-NeRF lack support for region-based transfer between identities.
This limitation arises from the fact that global-based representation such as tri-plane and MLP define all the 3D components in the 3D space.
Attempting a direct copy-paste of one tri-plane region to another results in inconsistencies, especially when there are variations in their absolute sizes.
% leads to inconsistency when their absolute size varies.

% \heading{FE-NeRF}
% Region-based editing or inversion.
\clearpage
